# Supplementary material for: Transition between Boundary-Limited Scaling and Mixing-Length Scaling of Turbulent Transport in Internally Heated Convection
Source: arXiv:2111.10906 ancillary file (2022-07-11)
Supplement: Supplementary file 1 [file sinansupp.pdf]

# Supplemental material:
# Transition between boundary-limited and mixing-length scalings of turbulent transport in internally heated convection


Sina Kazemi
*Department of Mechanical Engineering, University of Houston, Houston, TX 77040, USA*

David Goluskin
*Department of Mathematics and Statistics University of Victoria, Victoria, BC V8P 5C2*

Rodolfo Ostilla-Mónico
*Department of Mechanical Engineering, University of Houston, Houston, TX 77040, USA and*
*Escuela Superior de Ingenería, Universidad de Cádiz, Cádiz, Spain*



(Dated: May 23, 2022)


| | Uniform heating | $\ell = 0.05$, $\beta = 0$ | $\ell = 0.1$, $\beta = 0$ | $\ell = 0.1$, $\beta = 0.5$ | $\ell = 0.1$, $\beta = 0.7$ | $\ell = 0.1$, $\beta = 0.9$ | $\ell = 0.1$, $\beta = 1$ |
|---|---|---|---|---|---|---|---|
| $T_{st}(0)$ | 0.50 | 0.95 | 0.90 | 0.65 | 0.55 | 0.45 | 0.40 |
| $\langle T_{st} \rangle$ | 0.33 | 0.50 | 0.49 | 0.32 | 0.26 | 0.19 | 0.16 |
| $\alpha$ | 0.29 | 0.32 | 0.32 | 0.34 | 0.37 | 0.44 | 0.51 |
| $\gamma$ | 0.28 | 0.27 | 0.27 | 0.27 | 0.27 | 0.31 | – |

TABLE I. Heat transport properties for IHC with uniform heating or with an exponential heating/cooling profile of length scale $\ell$ and cooling strength $\beta$. For the dimensionless temperature profile $T_{st}(z)$ of the static state, the first two rows show the bottom temperature $T_{st}(0)$ and the mean temperature $\langle T_{st} \rangle$, respectively. The third row shows the best-fit exponent of the relation $Nu \approx c\, Ra^{\alpha}$, where $Nu = T_{st}(0)/\overline{T}(0)$ and $Ra = R/Nu$. The fourth row shows the best-fit exponent of the relation $\widetilde{Nu} \approx c\, \widetilde{Ra}^{\gamma}$, where $\widetilde{Nu} = \langle T_{st} \rangle / \langle T \rangle$ and $\widetilde{Ra} = R/\widetilde{Nu}$. No $\gamma$ is reported for the $\beta = 1$ case because $\langle T \rangle$ values are near zero and do not follow a power law.

| | $R$ | $\Gamma$ | $N_\Gamma^2 \times N_z$ | $t$ | $\overline{T}(0)$ | $\langle T \rangle$ | $Re$ | $Nu$ | $Ra$ |
|---|---|---|---|---|---|---|---|---|---|
| Uniform Heating | $10^5$ | $\pi$ | $288^2 \times 144$ | $2.108 \times 10^2$ | $1.678 \times 10^{-1}$ | $1.544 \times 10^{-1}$ | $2.622 \times 10^1$ | $2.979 \times 10^0$ | $3.356 \times 10^4$ |
| | $10^6$ | $\pi$ | $288^2 \times 144$ | $5.900 \times 10^1$ | $1.038 \times 10^{-1}$ | $9.998 \times 10^{-2}$ | $6.699 \times 10^1$ | $4.815 \times 10^0$ | $2.077 \times 10^5$ |
| | $10^7$ | 2.0 | $240^2 \times 144$ | $3.162 \times 10^1$ | $6.412 \times 10^{-2}$ | $6.401 \times 10^{-2}$ | $1.613 \times 10^2$ | $7.798 \times 10^0$ | $1.282 \times 10^6$ |
| | $10^8$ | 1.5 | $360^2 \times 240$ | $3.838 \times 10^0$ | $3.888 \times 10^{-2}$ | $3.905 \times 10^{-2}$ | $3.766 \times 10^2$ | $1.286 \times 10^1$ | $7.775 \times 10^6$ |
| | $10^9$ | 1.0 | $576^2 \times 576$ | $1.018 \times 10^{-2}$ | $2.207 \times 10^{-2}$ | $2.220 \times 10^{-2}$ | $8.131 \times 10^2$ | $2.265 \times 10^1$ | $4.414 \times 10^7$ |
| | $10^{10}$ | 1.0 | $576^2 \times 576$ | $4.480 \times 10^{-3}$ | $1.286 \times 10^{-2}$ | $1.279 \times 10^{-2}$ | $1.863 \times 10^3$ | $3.887 \times 10^1$ | $2.573 \times 10^8$ |
| $\ell = 0.05, \beta = 0$ | $10^5$ | $\pi$ | $288^2 \times 144$ | $1.522 \times 10^2$ | $2.358 \times 10^{-1}$ | $1.412 \times 10^{-1}$ | $3.692 \times 10^1$ | $4.463 \times 10^0$ | $2.241 \times 10^4$ |
| | $10^6$ | $\pi$ | $288^2 \times 144$ | $4.028 \times 10^1$ | $1.391 \times 10^{-1}$ | $8.808 \times 10^{-2}$ | $9.611 \times 10^1$ | $7.566 \times 10^0$ | $1.322 \times 10^5$ |
| | $10^7$ | 2.0 | $240^2 \times 144$ | $1.878 \times 10^1$ | $7.584 \times 10^{-2}$ | $5.335 \times 10^{-2}$ | $2.383 \times 10^2$ | $1.388 \times 10^1$ | $7.205 \times 10^5$ |
| | $10^8$ | 1.5 | $360^2 \times 240$ | $3.888 \times 10^0$ | $4.331 \times 10^{-2}$ | $3.242 \times 10^{-2}$ | $5.342 \times 10^2$ | $2.430 \times 10^1$ | $4.114 \times 10^6$ |
| | $10^9$ | 1.0 | $576^2 \times 576$ | $9.700 \times 10^{-1}$ | $2.497 \times 10^{-2}$ | $2.018 \times 10^{-2}$ | $1.076 \times 10^3$ | $4.216 \times 10^1$ | $2.372 \times 10^7$ |
| | $10^{10}$ | 1.0 | $576^2 \times 576$ | $3.041 \times 10^{-1}$ | $1.425 \times 10^{-2}$ | $1.217 \times 10^{-2}$ | $2.564 \times 10^3$ | $7.385 \times 10^1$ | $1.354 \times 10^8$ |
| $\ell = 0.1, \beta = 0$ | $10^5$ | $\pi$ | $288^2 \times 144$ | $2.093 \times 10^2$ | $2.103 \times 10^{-1}$ | $1.420 \times 10^{-1}$ | $3.674 \times 10^1$ | $5.283 \times 10^0$ | $1.893 \times 10^4$ |
| | $10^6$ | $\pi$ | $288^2 \times 144$ | $6.666 \times 10^1$ | $1.239 \times 10^{-1}$ | $9.040 \times 10^{-2}$ | $9.505 \times 10^1$ | $8.965 \times 10^0$ | $1.115 \times 10^4$ |
| | $10^7$ | 2.0 | $240^2 \times 144$ | $3.041 \times 10^1$ | $6.864 \times 10^{-2}$ | $5.529 \times 10^{-2}$ | $2.352 \times 10^2$ | $1.619 \times 10^1$ | $6.178 \times 10^5$ |
| | $10^8$ | 1.5 | $360^2 \times 240$ | $3.895 \times 10^0$ | $4.017 \times 10^{-2}$ | $3.419 \times 10^{-2}$ | $5.326 \times 10^2$ | $2.766 \times 10^1$ | $3.615 \times 10^6$ |
| | $10^9$ | 1.0 | $576^2 \times 576$ | $2.866 \times 10^0$ | $2.329 \times 10^{-2}$ | $2.022 \times 10^{-2}$ | $1.063 \times 10^3$ | $4.770 \times 10^1$ | $2.096 \times 10^7$ |
| | $10^{10}$ | 1.0 | $576^2 \times 576$ | $1.305 \times 10^0$ | $1.326 \times 10^{-2}$ | $1.210 \times 10^{-2}$ | $2.482 \times 10^3$ | $8.376 \times 10^1$ | $1.194 \times 10^8$ |
| $\ell = 0.1, \beta = 0.5$ | $10^5$ | $\pi$ | $288^2 \times 144$ | $6.660 \times 10^1$ | $1.529 \times 10^{-1}$ | $8.00 \times 10^{-2}$ | $3.189 \times 10^1$ | $1.006 \times 10^1$ | $9.941 \times 10^3$ |
| | $10^6$ | $\pi$ | $288^2 \times 144$ | $3.447 \times 10^1$ | $8.561 \times 10^{-2}$ | $4.844 \times 10^{-2}$ | $8.429 \times 10^1$ | $1.797 \times 10^1$ | $5.565 \times 10^4$ |
| | $10^7$ | 2.0 | $240^2 \times 144$ | $1.544 \times 10^1$ | $4.510 \times 10^{-2}$ | $2.830 \times 10^{-2}$ | $2.104 \times 10^2$ | $3.411 \times 10^1$ | $2.932 \times 10^5$ |
| | $10^8$ | 1.5 | $360^2 \times 240$ | $1.000 \times 10^1$ | $2.543 \times 10^{-2}$ | $1.802 \times 10^{-2}$ | $4.734 \times 10^2$ | $6.050 \times 10^1$ | $1.653 \times 10^6$ |
| | $10^9$ | 1.0 | $576^2 \times 576$ | $2.557 \times 10^0$ | $1.417 \times 10^{-2}$ | $1.123 \times 10^{-2}$ | $9.804 \times 10^2$ | $1.086 \times 10^2$ | $9.210 \times 10^6$ |
| | $10^{10}$ | 1.0 | $576^2 \times 576$ | $1.364 \times 10^0$ | $8.221 \times 10^{-2}$ | $6.718 \times 10^{-3}$ | $2.158 \times 10^3$ | $1.860 \times 10^2$ | $5.377 \times 10^7$ |

| | $R$ | $\Gamma$ | $N_\Gamma^2 \times N_z$ | $t$ | $\overline{T}(0)$ | $\langle T \rangle$ | $Re$ | $Nu$ | $Ra$ |
|---|---|---|---|---|---|---|---|---|---|
| $\ell = 0.1, \beta = 0.7$ | $10^5$ | $\pi$ | $288^2 \times 144$ | $1.328 \times 10^2$ | $1.270 \times 10^{-1}$ | $5.305 \times 10^{-2}$ | $2.941 \times 10^1$ | $1.432 \times 10^1$ | $6.984 \times 10^3$ |
| | $10^6$ | $\pi$ | $288^2 \times 144$ | $1.520 \times 10^1$ | $6.818 \times 10^{-2}$ | $3.034 \times 10^{-2}$ | $7.810 \times 10^1$ | $2.667 \times 10^1$ | $3.750 \times 10^4$ |
| | $10^7$ | 2.0 | $240^2 \times 144$ | $2.458 \times 10^1$ | $3.515 \times 10^{-2}$ | $1.650 \times 10^{-2}$ | $1.917 \times 10^2$ | $5.172 \times 10^1$ | $1.934 \times 10^5$ |
| | $10^8$ | 1.5 | $360^2 \times 240$ | $9.661 \times 10^0$ | $1.881 \times 10^{-2}$ | $1.099 \times 10^{-2}$ | $4.340 \times 10^2$ | $9.665 \times 10^1$ | $1.035 \times 10^6$ |
| | $10^9$ | 1.0 | $576^2 \times 576$ | $3.048 \times 10^0$ | $1.040 \times 10^{-2}$ | $7.163 \times 10^{-3}$ | $9.221 \times 10^2$ | $1.748 \times 10^2$ | $5.719 \times 10^6$ |
| | $10^{10}$ | 1.0 | $576^2 \times 576$ | $4.814 \times 10^{-1}$ | $5.881 \times 10^{-2}$ | $4.423 \times 10^{-3}$ | $2.159 \times 10^3$ | $3.091 \times 10^2$ | $3.235 \times 10^7$ |
| $\ell = 0.1, \beta = 0.9$ | $10^5$ | $\pi$ | $288^2 \times 144$ | $1.319 \times 10^2$ | $9.810 \times 10^{-2}$ | $2.394 \times 10^{-2}$ | $2.654 \times 10^1$ | $2.265 \times 10^1$ | $4.415 \times 10^3$ |
| | $10^6$ | $\pi$ | $288^2 \times 144$ | $4.513 \times 10^1$ | $5.137 \times 10^{-2}$ | $1.128 \times 10^{-2}$ | $7.008 \times 10^1$ | $4.326 \times 10^1$ | $2.311 \times 10^4$ |
| | $10^7$ | 2.0 | $240^2 \times 144$ | $1.560 \times 10^1$ | $2.524 \times 10^{-2}$ | $4.757 \times 10^{-3}$ | $1.691 \times 10^2$ | $8.804 \times 10^1$ | $1.136 \times 10^5$ |
| | $10^8$ | 1.5 | $360^2 \times 240$ | $8.870 \times 10^0$ | $1.205 \times 10^{-2}$ | $2.965 \times 10^{-3}$ | $4.007 \times 10^2$ | $1.844 \times 10^2$ | $5.422 \times 10^5$ |
| | $10^9$ | 1.0 | $576^2 \times 576$ | $2.530 \times 10^0$ | $6.016 \times 10^{-3}$ | $1.512 \times 10^{-3}$ | $8.648 \times 10^2$ | $3.694 \times 10^2$ | $2.707 \times 10^6$ |
| | $10^{10}$ | 1.0 | $576^2 \times 576$ | $1.000 \times 10^0$ | $2.934 \times 10^{-3}$ | $6.120 \times 10^{-4}$ | $1.966 \times 10^3$ | $7.574 \times 10^2$ | $1.320 \times 10^7$ |
| $\ell = 0.1, \beta = 1.0$ | $10^5$ | $\pi$ | $288^2 \times 144$ | $6.618 \times 10^1$ | $8.667 \times 10^{-2}$ | $1.009 \times 10^{-2}$ | $2.517 \times 10^1$ | $2.918 \times 10^1$ | $3.427 \times 10^3$ |
| | $10^6$ | $\pi$ | $288^2 \times 144$ | $4.818 \times 10^1$ | $4.246 \times 10^{-2}$ | $2.409 \times 10^{-3}$ | $6.621 \times 10^1$ | $5.858 \times 10^1$ | $1.707 \times 10^4$ |
| | $10^7$ | 2.0 | $240^2 \times 144$ | $1.993 \times 10^1$ | $2.067 \times 10^{-2}$ | $-8.107 \times 10^{-4}$ | $1.595 \times 10^2$ | $1.220 \times 10^2$ | $8.199 \times 10^4$ |
| | $10^8$ | 1.5 | $360^2 \times 240$ | $1.291 \times 10^1$ | $8.894 \times 10^{-3}$ | $-6.664 \times 10^{-4}$ | $3.797 \times 10^2$ | $2.768 \times 10^2$ | $3.613 \times 10^5$ |
| | $10^9$ | 1.0 | $576^2 \times 576$ | $5.998 \times 10^0$ | $3.694 \times 10^{-3}$ | $1.161 \times 10^{-5}$ | $8.192 \times 10^2$ | $6.917 \times 10^2$ | $1.446 \times 10^6$ |
| | $10^{10}$ | 1.0 | $576^2 \times 576$ | $9.500 \times 10^{-1}$ | $1.841 \times 10^{-3}$ | $1.475 \times 10^{-4}$ | $1.889 \times 10^3$ | $1.367 \times 10^3$ | $7.317 \times 10^7$ |

TABLE II: Simulation parameters and mean quantities. The parameters $R$ and horizontal-to-vertical aspect ratio $\Gamma$ are varied while $Pr = 1$ is fixed. Simulations use a mesh with $N_\Gamma$ points in the horizontal directions and $N_z$ in the vertical, and averages are taken over $t$ thermal diffusive time units. The time-averaged quantities reported are the bottom temperature $\overline{T}(0)$, the volume-averaged temperature $\langle T \rangle$, the Reynolds number $Re = dU/\nu$ with the dimensional velocity scale $U$ being the root-mean-squared velocity magnitude, the Nusselt number $Nu$, and the diagnostic Rayleigh number $Ra = R/Nu$.

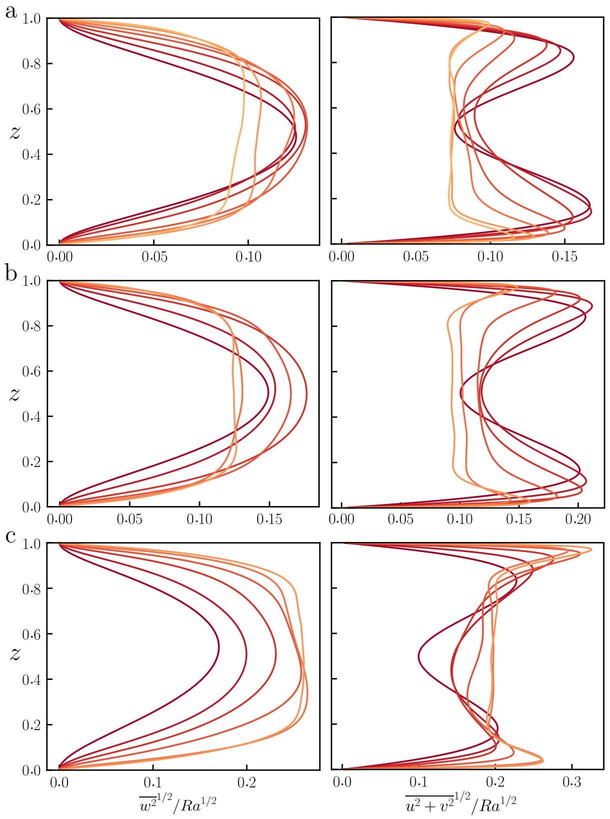


FIG. 1. Horizontally and temporally averaged profiles of root-mean-squared vertical velocity (left) and horizontal velocity (right) at $R = 10^5, 10^6, 10^7, 10^8, 10^9, 10^{10}$ (dark to light), compensated by $Ra^{1/2}$, for (a) uniform heating, (b) exponentially distributed heating with $(\ell, \beta) = (0.1, 0)$, and (c) net-zero heating/cooling with $(\ell, \beta) = (0.1, 1)$.

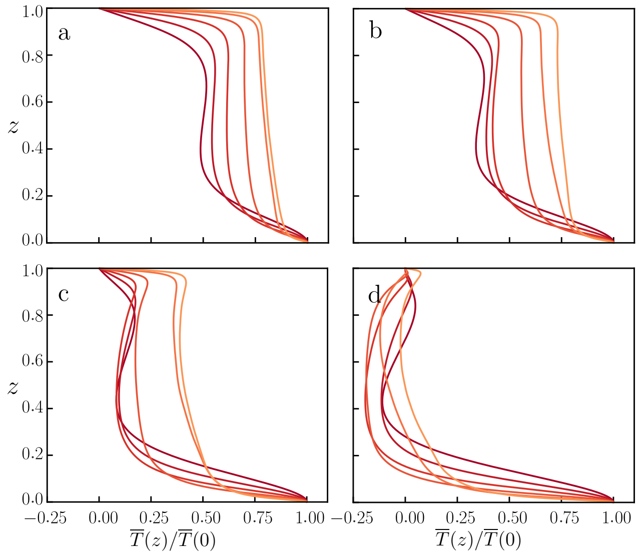


FIG. 2. Horizontally and temporally averaged normalized temperature profiles at $R = 10^5, 10^6, 10^7, 10^8, 10^9, 10^{10}$ (dark to light), normalized by the mean bottom temperature $\overline{T}(0)$, for exponentially distributed heating/cooling with $\ell = 0.1$ and (a) $\beta = 0.5$, (b) $\beta = 0.7$, (c) $\beta = 0.9$, and (d) $\beta = 1$.
